# Supplementary material for: Positive helicity Einstein-Yang-Mills amplitudes from the Double Copy
Source: arXiv:1812.04053 source file (2019-01-19)

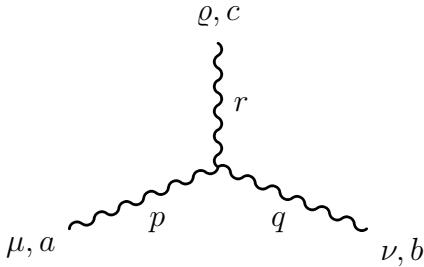

$\mu, a$

$\sigma, d$

$\nu, b$

$\varrho, c$

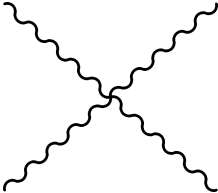

$C, c$

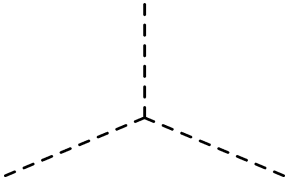

$A, a$

$B, b$

$A, a$

$D, d$

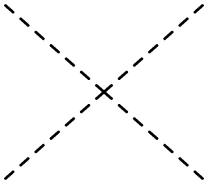

$B, b$

$C, c$

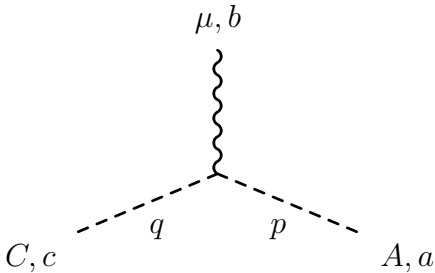

$D, d$

$\nu, c$

$\mu, a$

$B, b$

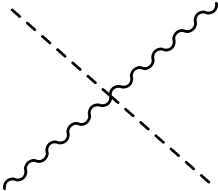

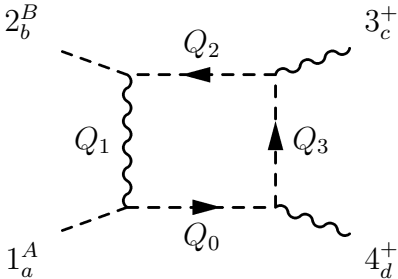

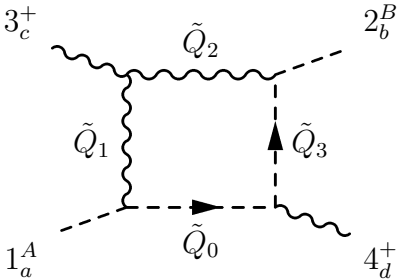



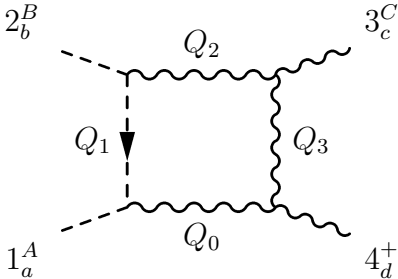

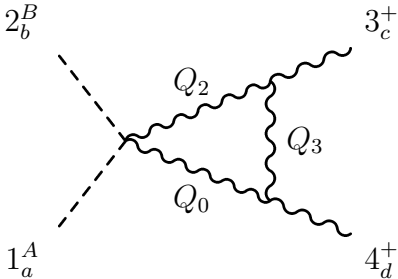

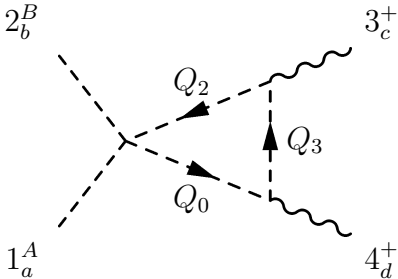

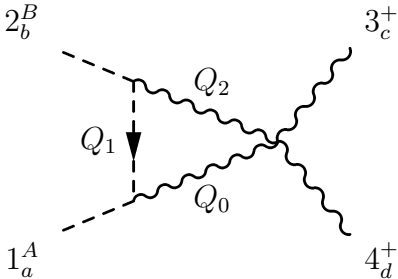

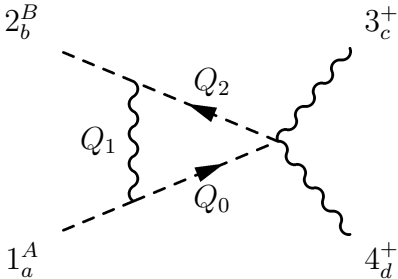

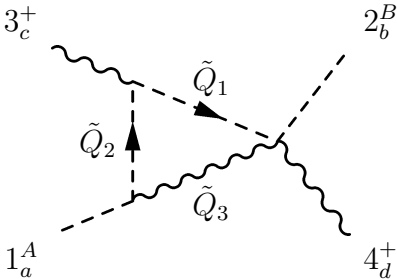

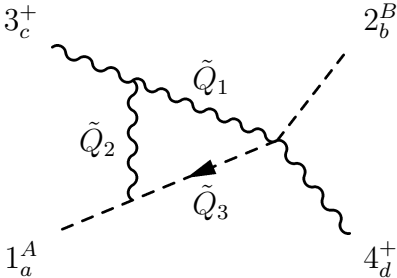

Supplement: Supplementary file 1 [file PicAppendix.pdf]
